# Supplementary material for: Learning from Multiway Data: Simple and Efficient Tensor Regression
Source: arXiv:1607.02535 source file (2016-07-08)
Supplement: Supplementary file 1 [file appendix_model.tex]

Given the fact that $\text{vec}(ABC) = (C^T \otimes A) \text{vec}(B)$, we have  
$\text{vec}(Y_m) =\text{vec}(\T{X}_m \T{W}_m)  =  (I_P \otimes \T{X}_m) \text{vec}(\T{W}_m) $. For the complete model, 
$\text{vec}(\T{Y})   =  \text{diag}( I_P \otimes  \T{X}) \text{vec}(\T{W}_m) $, where $\text{diag}(I_P \otimes \T{X}) =  \begin{bmatrix}
I_P \otimes\T{X}_{1}       & 0 & 0 & \dots & 0 \\
0      & I_P \otimes \T{X}_{2} & 0& \dots &0\\
\hdotsfor{5} \\
0     & 0 & 0 & \dots & I_P \otimes   \T{X}_{m}
\end{bmatrix}$.

For a tensor $\T{W}$ with Tucker decomposition $\T{W} =\M{S} \times_1 \M{U}_1 \times_2 \M{U}_2 \cdots \times_N \M{U}_M$ we have the  following two properties:  
\begin{enumerate}[(a)]
\item $\text{vec}(\T{W}) = (\M{U}_1 \otimes \M{U}_2  \otimes \cdots \otimes \M{U}_N )^T \text{vec}(\M{S}) $. 
\item  $\T{W}_{(n)} =  \M{U}_n \T{S}_{(n)} (\M{U}_N \otimes \cdots \M{U}_{n+1} \otimes \M{U}_{n-1} \cdots \otimes \M{U}_1) ^T$
\end{enumerate}

\paragraph{Greedy}
For rank-1 matching pursuit algorithm. The idea is to find the best rank-1 estimation and greedily add it to the existing solution. 
 For each variable $m$, our problem is an independent multivariate regression problem 
 $\frac{1}{2}\|\M{Y}_m -  \M{X}_m \M{W}_m\|_F^2$. Alternatively, denote $\M{\tilde{W}} = \T{W}_{(2)}^T$, the problem can be written as 
 \begin{eqnarray}
 \argmin\limits_{\text{rank}(\M{\tilde{W}} \leq R_2)}	\frac{1}{2} \| \M{\tilde{Y}}-  \M{\tilde{X}\M{\tilde{W}}} \|_2^F,  
 \end{eqnarray}
 where $\M{\tilde{Y}} = \T{Y}_{(2)}^T  $, $\M{\tilde{X}} =  \begin{bmatrix}
 	\M{X}_{1}       & 0 & 0 & \dots & 0 \\
 	0      & \M{X}_{2} & 0& \dots &0\\
 	\hdotsfor{5} \\
 	0     & 0 & 0 & \dots &  \M{X}_{m} 
 	\end{bmatrix}$ 
 	
This is a similar generalization from 2-way to 3-way as from 1-way to 2-way through concatenation.  With property  (a), we have $\M{\tilde{W}} =   (\M{U}_N \otimes \cdots \M{U}_{n+1} \otimes \M{U}_{n-1} \cdots \otimes \M{U}_1) \T{S}_{(n)}^T \M{U}_n^T $.  Find the best rank-1 component of the above problem leads to the following optimization problem, which can be solved efficiently using alternating direction method. ( This is a bi-convex problem, thus local optimal solution???)
\begin{eqnarray}
	 \argmin\limits_{\alpha, \V{u}, \V{v} }	\frac{1}{2} \| \M{\tilde{Y}}-  \M{\tilde{X}}  \alpha\V{u}\V{v}^T \|_2^F,  
\end{eqnarray}
$\V{u} = \text{eigs}(\M{\tilde{X}}^T\M{\tilde{X}} , \M{\tilde{X}}^T \M{\tilde{Y}}\M{\tilde{Y}}^T \M{\tilde{X}})$,  $\V{v} =   \M{\tilde{Y}} ^T  \M{\tilde{X}} \V{u} / \| \M{\tilde{Y}} ^T  \M{\tilde{X}} \V{u} \|$ and  $\alpha = (\V{X}\V{u}\V{v})^T \M{\tilde{Y}} / \| (\V{X}\V{u}\V{v})^T \|\M{\tilde{Y}}\|$, 
The algorithm proceeds by greedily adding the rank-1 component from one of the modes. Actually, all the modes are equivalent. To see this,  suppose we obtain a decomposition on mode-1, $\W_{(1)}= \alpha_1 \V{u}_1 \V{v}_1^T$ with $\V{u}_1 \in \R^{Q\times 1}$ and $\V{v}_1 \in \R^{PM\times 1}$ \footnote{ 
	The uniqueness of rank-1 SVD depends on whether the largest singular value is distinct/de-generate or not}, now we want to find the decomposition on mode-2, i.e, $\W_{(2)}= \alpha_2 \V{u}_2 \V{v}_2^T$ where $\V{u}_2 \in \R^{P\times 1}$ and $\V{v}_2 \in \R^{QM\times 1}$. Write  $\V{v}_1 = [\V{v}_{1,1},\cdots, \V{v}_{1,m}, \cdots,\V{v}_{1,M}]$, $\V{v}_2 =  [\V{v}_{2,1},\cdots, \V{v}_{2,m}, \cdots,\V{v}_{2,M}] $. It can be easily seen that $\alpha_1 \V{u}_1 \V{v}_{1,m} ^T =  \alpha_2 \V{v}_{2,m} \V{u}_2^T$. 

\paragraph{HOSVD}
 HOSVD \cite{de2000multilinear}  provides an equivalent representation of high-order generalization of singular value decompostion (SVD) as the SVD of the matrix unfoldings. When the  In tensor regression scenario,  We first obtain a least square estimation and then apply truncated HOSVD (T-HOSVD) on the resulting LS solution
%For CP model,  $\W= \sum_{r = 1}^R \sigma_r \V{u}^r_1 \otimes \V{u}^r_2 \cdots  \otimes  \V{u}^r_N$, rank-1 component is 
\begin{algorithm}[h]
		\caption{ T-HOSVD for Tensor Regression }
		\label{alg:sketching}
		\begin{algorithmic}[1]
	\STATE Compute least square estimate  $\W^{LS}$ 
		\FOR{$n=1$ {\bfseries to} $N$}
		\STATE Compute SVD  of the matrix unfolding \\ $ \M{U}_n \M{\Sigma}_n\M{V}_n^T =\W_{(n)}$ 
	\ENDFOR
		\STATE Compute core tensor  \\ $\M{S} = \T{W}^{LS} \times_1 \M{U}_{1(1:R,:)}^T\cdots \times_N \M{U}_{N(1:R,:)}^T$
	\STATE Compute low-rank estimation \\ $\widehat{\W} = \M{S} \times_1 \M{U}_{1(1:R,:)}\cdots \times_N \M{U}_{N(1:R,:)} $
	\end{algorithmic}
\end{algorithm}
It is known that truncated HOSVD maybe sub-optimal for the best rank-R approximation. 

% Approximation analysis
Let the objective function be 
\begin{eqnarray}
	\frac{1}{2}  \text{tr} \{ \sum_{i=m }^M (\M{Y}_m -  \M{X}_m \M{W}_m)^T (\M{Y}_m -  \M{X}_m \M{W}_m)   \} + \lambda  \M{\Sigma}(\W)
\end{eqnarray}
where $\Sigma(\W)$ denotes the singular values of the $\W$ obtained from HOSVD.
\begin{eqnarray*}
& \text{tr} \{ \sum_{i=m }^M (\M{Y}_m -  \M{X}_m \M{W}_m)^T (\M{Y}_m -  \M{X}_m \M{W}_m) \} \\
= &  \sum_{i=m }^M    \text{tr} \{ (\M{Y}_m -  \M{X}_m \M{W}^{LS}_m)^T (\M{Y}_m -  \M{X}_m \M{W}^{LS}_m) \} \\
+ &  \text{tr} \{ (\M{W}^{LS}_m - \M{W}_m  )^T  \M{X}_m^T  \M{X}_m(\M{W}^{LS}_m - \M{W}_m  )  \} \\
= & \text{tr} \{ (\tilde{\M{Y}} -  \tilde{\M{X}}  \tilde{\M{W}}^{LS})^T (\tilde{\M{Y}} -  \tilde{\M{X}}  \tilde{\M{W}}^{LS}) \} \\
+ &  \text{tr} \{ (\tilde{\M{W}}^{LS} - \tilde{\M{W}}  )^T  \tilde{\M{X}}^T  \tilde{\M{X}} (\tilde{\M{W}}^{LS} - \tilde{\M{W}}  )  \}
\end{eqnarray*}
Note that $\text{tr}( \tilde{\M{W}}^T  \tilde{\M{W}}  ) =  \text{tr}( \tilde{\M{W}} \tilde{\M{W}}^T) = \text{tr}\{(\M{\Sigma}^{(2)}  )^2\} = \sum_{i = 1}^{\min\{P,Q\}} (\sigma^{(2)}_i)^2$.
Thus the loss function becomes
\begin{eqnarray*}
	\frac{1}{2}  \text{tr}\{ \tilde{\M{X}}^T  \tilde{\M{X}} ( \M{\Sigma}^{(2)}  )^2\} - \text{tr}\{ \tilde{\M{X}}^T  \tilde{\M{X}}   \tilde{\M{W}}^{LS}  \tilde{\M{W}}     \} + \lambda \M{\Sigma}(\W)
\end{eqnarray*}

Now analyze the error between T-HOSVD vs the optimal $\W$
\begin{eqnarray*}
&\tilde{\M{W}} ^{LS}  &=  (\tilde{\M{X}}^T  \tilde{\M{X}})^{-1}(\tilde{\M{X}}^T \tilde{\M{Y}}) \\
& = & (\tilde{\M{X}}^T  \tilde{\M{X}})^{-1}\tilde{\M{X}}^T (\tilde{\M{X}} \tilde{\M{W}} + \M{E}) \\
& = & \tilde{\M{W}}  + \tilde{\M{X}}^{-1} \M{E} 
\end{eqnarray*}

$\M{E}$ has i.i.d entires from standard normal distribution. Given that  $\tilde{\M{W}}= \W_{(2)}^T$, let $\W^{LS} = refold( (\tilde{\M{W}}_{LS})^T,2)$ the equivalent tensor representation is 
\begin{eqnarray*}
	\W^{LS} = \W  + \X^{-1}\E
\end{eqnarray*}
define the estimation  $\widehat{\T{W}} $ as the result of iteratively finding the orthogonal singular vectors of $\W^{LS}$ for all modes $\M{U}^{(n)LS} = [\V{u}_1^{(n)LS}, \V{u}_2^{(n)LS},\cdots, \V{u}_{R_n}^{(n)LS} ]$, which boils down to solving the following eigenvalue problem. 
\begin{eqnarray*}
	\end{eqnarray*}

Eigenvalue perturbation: 

The truncated HOSVD solution $\widehat{\T{W}}$, though not the best approximation under the n-mode rank constraints (24) in \cite{de2000multilinear} , is still a good approximation with bounded error. \\
